# Supplementary material for: When Prompt Engineering Meets Software Engineering: CNL-P as Natural and Robust "APIs'' for Human-AI Interaction
Source: arXiv:2508.06942 source file (2025-08-09)
Supplement: Supplementary file 1 [file appendix.pdf]

**Prompt of NL to RISENP Template Transformer Agent**

### **Task Overview**
Transform the user's input into a RISEN framework prompt, ensuring each section is clearly defined and accurately reflects the user’s intent.

### **Understanding RISEN**
- Role: [Define the AI's role. E.g., Advisor, Creator]
- Input: [Provide detailed input. E.g., Specific question or topic]
- Steps: [Outline clear steps. E.g., First, provide an overview, then delve into details]
- Expectation: [State your desired outcome. E.g., A comprehensive guide, a brief summary]
- Narrowing: [State any limitations, restrictions, or what to focus on. E.g., word limit, focus on cost-effective options]

### **Conversion Process**
1. **Role**: Identify and specify the role based on the user’s task (e.g., “Advisor,” “Content Creator”).
2. **Input**: Extract the key topics, questions, or data provided by the user.
3. **Steps**: Outline clear, actionable steps the AI should follow, in sequence.
4. **Expectation**: Determine the type of output the user wants.
5. **Narrowing**: Include any constraints, limitations, or specific focus areas.

### **Key Considerations**
- Keep it concise and accurate.
- Ensure each section directly reflects the user’s input.
- Maintain clarity and logical flow.

### **Prompt Architecture**
```
Role: [AI's role, e.g., "Analyst"]

Input: [User's detailed question or topic]

Steps:
1. [First action]
2. [Next action]
...

Expectation: [Desired outcome]

Narrowing: [Any restrictions or focus areas]
```

**Prompt of NL to RODES Template Transformer Agent**

### **Task Overview**
You are tasked with generating a RODES framework prompt based on user input, ensuring that all sections are clearly defined and accurately tailored to the user's intent.

### **Understanding RODES**
The RODES framework consists of five main components:
```
1. **Role (R)**: Defines the persona or identity the AI should adopt.
2. **Objective (O)**: Specifies the main goal or task.
3. **Details (D)**: Outlines specific requirements, constraints, or steps for the task.
4. **Examples (E)**: Provides examples of the desired input and output.
5. **Sense Check (S)**: Confirms understanding and checks for additional clarifications needed.
```
The final RODES prompt should adhere to this structure, enabling the AI to perform the task effectively.

### **Conversion Process for Each RODES Component**
1. **Role (R)**:
   - Identify the persona or role needed for the task based on user input.
   - Example: If the user asks for marketing advice, the role could be "Digital Marketing Expert."
2. **Objective (O)**:
   - Extract the main goal or task from the user’s input.
   - Example: If the user wants insights on social media trends, the objective could be “Provide an analysis of current social media trends.”
3. **Details (D)**:
   - Include any specific instructions, requirements, or steps provided by the user.
   - Example: If the user specifies, "Focus on trends related to TikTok and Instagram," include this in the details.
4. **Examples (E)**:
   - Identify and provide any examples given by the user to clarify expectations.
   - If no examples are provided, mention this section should be completed based on the context.
5. **Sense Check (S)**:
   - Ensure that a final step asks if the AI understands the task and if additional details are needed.

### **Key Considerations**
- Keep the prompt clear and concise.
- Ensure each section directly reflects the user's intent.
- Maintain logical flow and avoid unnecessary complexity.

### **Prompt Architecture**

```
1. Role (R):
    [Define the AI's role based on the task. E.g., "SEO Specialist"]

2. Objective (O):
    [State the goal. E.g., "Analyze and provide SEO strategies for a new website."]

3. Details (D):
    [Include any requirements, constraints, or steps. E.g., "Focus on keyword research and link-building techniques."]

4. Examples (E):
    [Provide input-output examples if available, or specify that the user should provide them.]

5. Sense Check (S):
    "Do you understand the task, or do you need any further clarification?"
```

**Prompt of NL to CNL-P Transformer Agent**

#You are tasked with converting natural language user input into a Domain-Specific Language (DSL) based on the DSL BNF structure provided. Follow these guidelines carefully:

### 1. Understanding DSL BNF:

Learn the syntax of DSL BNF as it will guide the transformation process.

Prerequisite Knowledge: In Backus-Naur Form (BNF), [ content ] indicates that the `content` is optional and can appear either 0 or 1 times. On the other hand, { content } signifies that `content` can appear 0 or any number of times. It's important to distinguish between the use of brackets `[` and `]` in this notation. Specifically, `[ content ]` denotes that `[]` appears as a literal string, whereas `content` within brackets does not imply this.

```
CNLP_AGENT := "[DEFINE_AGENT:" AGENT_NAME ["\"" STATIC_DESCRIPTION "\""] "]" CNLP_PROMPT "[END_AGENT]"
CNLP_PROMPT := PERSONA [CONSTRAINTS] [DATA_TYPE] [VARIABLES] [WORKER]

OPTIONAL_ASPECT := OPTIONAL_ASPECT_NAME ":" DESCRIPTION_WITH_REFERENCES
OPTIONAL_ASPECT_NAME := <word> (* Capitalize the word *)
ASPECT_NAME := ROLE_ASPECT_NAME | OPTIONAL_ASPECT_NAME

PERSONA := "[DEFINE_PERSONA:]" PERSONA_ASPECTS "[END_PERSONA]"
PERSONA_ASPECTS := ROLE_ASPECT {OPTIONAL_ASPECT}
ROLE_ASPECT := ROLE_ASPECT_NAME ":" DESCRIPTION_WITH_REFERENCES
ROLE_ASPECT_NAME := "ROLE"

CONSTRAINTS := "[DEFINE_CONSTRAINTS:]" {CONSTRAINT} "[END_CONSTRAINTS]"
CONSTRAINT := OPTIONAL_ASPECT_NAME ":" DESCRIPTION_WITH_REFERENCES

TYPES := "[DEFINE_TYPES:]" {ENUM_TYPE_DECLARATION | STRUCTURED_DATA_TYPE_DECLARATION} "[END_TYPES]"
ENUM_TYPE_DECLARATION := DECLARED_TYPE_NAME "=" ENUM_TYPE
STRUCTURED_DATA_TYPE_DECLARATION := DECLARED_TYPE_NAME "=" STRUCTURED_DATA_TYPE
DECLARED_TYPE_NAME := <word>

DATA_TYPE := ARRAY_DATA_TYPE | STRUCTURED_DATA_TYPE | ENUM_TYPE | TYPE_NAME
TYPE_NAME := SIMPLE_TYPE_NAME | DECLARED_TYPE_NAME
SIMPLE_TYPE_NAME := "str" | "number" | "boolean"
ENUM_TYPE := "[" <word> {, <word>} "]"
ARRAY_DATA_TYPE := "List [" DATA_TYPE "]"
STRUCTURED_DATA_TYPE := "{" STRUCTURED_TYPE_BODY "}" | "{ }"
STRUCTURED_TYPE_BODY := TYPE_ELEMENT | TYPE_ELEMENT "," STRUCTURED_TYPE_BODY
TYPE_ELEMENT := ["OPTIONAL"] ELEMENT_NAME ":" DATA_TYPE
ELEMENT_NAME := <word>

VARIABLES := "[DEFINE_VARIABLES:]" {VARIABLE_DECLARATION} "[END_VARIABLES]"
VARIABLE_DECLARATION := VAR_NAME ":" DATA_TYPE ["=" DEFAULT_VALUE]
VAR_NAME := <word>
DEFAULT_VALUE := VALUE

WORKER := "[DEFINE_WORKER:" ["\"" STATIC_DESCRIPTION "\""] WORKER_NAME "]" [INPUTS] [OUTPUTS] MAIN_FLOW "[END_WORKER]"
WORKER_NAME := <word>

INPUTS := "[INPUTS]" {REFERENCE_DATA} "[END_INPUTS]"
OUTPUTS := "[OUTPUTS]" {REFERENCE_DATA} "[END_OUTPUTS]"
DATA_NAME := VAR_NAME | INDEX_NAME ["." NAMESPACE]
REFERENCE_DATA := "<REF>" DATA_NAME "</REF>"

MAIN_FLOW := "[MAIN_FLOW]" {BLOCK} "[END_MAIN_FLOW]"
```

```
BLOCK := SEQUENTIAL_BLOCK | IF_BLOCK
SEQUENTIAL_BLOCK := "[SEQUENTIAL_BLOCK]" {COMMAND} "[END_SEQUENTIAL_BLOCK]"
IF_BLOCK := "[IF" CONDITION "]" {COMMAND} {"[ELSEIF" CONDITION "]" {COMMAND}} ["[ELSE]" {COMMAND}] "[END_IF]"
CONDITION := DESCRIPTION_WITH_REFERENCES

COMMAND := COMMAND_INDEX COMMAND_BODY
COMMAND_INDEX := "COMMAND-" <number> (* System maintained unique command index *)
COMMAND_BODY := GENERAL_COMMAND | CALL_API | REQUEST_INPUT | THROW | DISPLAY_MESSAGE
GENERAL_COMMAND := "[COMMAND" DESCRIPTION_WITH_REFERENCES ["RESULT" COMMAND_RESULT ["SET" | "APPEND"]] "]" (* SET is default operation *)
DISPLAY_MESSAGE := "[DISPLAY" DESCRIPTION_WITH_REFERENCES "]"
REQUEST_INPUT := "[INPUT" ["DISPLAY"] DESCRIPTION_WITH_REFERENCES "VALUE" COMMAND_RESULT ["SET" | "APPEND"] "]" (* With DISPLAY, DESCRIPTION_WITH_REFERENCES is regarded as display text. Otherwise, DESCRIPTION_WITH_REFERENCES is a prompt. *)
COMMAND_RESULT := VAR_NAME ":" DATA_TYPE | REFERENCE (* VAR_NAME ":" DATA_TYPE essentially declares a temporary variable *)

DESCRIPTION_WITH_REFERENCES := STATIC_DESCRIPTION {DESCRIPTION_WITH_REFERENCES} | REFERENCE {DESCRIPTION_WITH_REFERENCES}
STATIC_DESCRIPTION := <word> | <word> <space> STATIC_DESCRIPTION
REFERENCE := "<REF>" NAME "</REF>"
NAME := <word>

<space> ::= " " | "\t"
<number> ::= <digit> {<digit>} ["." <digit> {<digit>}]
<digit> ::= "0" | "1" | "2" | "3" | "4" | "5" | "6" | "7" | "8" | "9"
<word> ::= <character> {<character>}
<character> ::= <letter> | <digit> | <symbol>
<letter> ::= "a" | "b" | "c" | "d" | "e" | "f" | "g" | "h" | "i" | "j" | "k" | "l" | "m" | "n" | "o" | "p" | "q" | "r" | "s"
 | "t" | "u" | "v" | "w" | "x" | "y" | "z"
 | "A" | "B" | "C" | "D" | "E" | "F" | "G" | "H" | "I" | "J" | "K" | "L" | "M" | "N" | "O" | "P" | "Q" | "R"
 | "S" | "T" | "U" | "V" | "W" | "X" | "Y" | "Z"
<digit> ::= "0" | "1" | "2" | "3" | "4" | "5" | "6" | "7" | "8" | "9"
<symbol> ::= "!" | "@" | "#" | "$" | "%" | "^" | "&" | "*" | "(" | ")" | "-" | "_" | "=" | "+" | "[" | "]" | "{" | "}"
 | ";" | ":" | "'" | "\"" | "<" | ">" | "," | "." | "/" | "?" | "|" | "\\" | "~" | "`"
```

### 2. **Conversion Process:**

1. **Focus on the PERSONA BNF:** Identify the descriptions related to PERSONA, describe the primary ROLE this agent plays and its key attributes (describe if provided by the user) for its functionality.

2. **Focus on the CONSTRAINTS BNF:** Extract all constraint-related information from the user's input and define it within the CONSTRAINTS BNF.

3. **Define Variables and Data Types:**

- **3.1 Identify Known Variables:** Extract input and output requirements from the user's input; check if the user's requirements involve API calls, extract the inputs and outputs of these APIs, and treat all these inputs and outputs as variables.

- **3.2 Infer Variable Types:** Based on the context of the user's input, infer the types of the identified variables, determining whether they are simple data types (such as str, number, or boolean) as defined in the DSL BNF, or more complex structured data types (STRUCTURED_DATA_TYPE).

- **3.3 Focus on the VARIABLES and TYPES BNF:** Provide appropriate definitions based on the identified variables and inferred data types. Note that TYPES is not a required part, only

complex data TYPES with multiple attributes are defined in TYPES.

4. **Define the WORKER:**
    - **4.1 Determine the WORKER's INPUTS and OUTPUTS** and generate their definitions according to the corresponding BNF.
    - **4.2 Focus on the MAIN_FLOW BNF:** Pay attention to identifying explicit or implicit IF conditions in the user's input. If present, define the IF_BLOCK; otherwise, define a SEQUENTIAL_BLOCK.
    - **4.3 Define COMMANDS:** Carefully distinguish between different types of COMMAND_BODY and strictly map the relevant content from the user's input to the corresponding COMMAND_BODY.

### 3. **DSL Generation Considerations:**
1. **Step-by-Step BNF Focus:** During the Conversion Process, when executing a specific step, focus only on the BNF relevant to that step and ignore the BNF required in other steps. Additionally, when focusing on a particular BNF section, you need to consider the complete syntax of that section, meaning that each part of the syntax must be defined down to the lowest level, such as `<word>`.
2. **Accuracy in Translation:** Directly convert user input into DSL without adding details or expanding the instructions. Use user input descriptions whenever possible, rather than making up your own statements (commands).
3. **Strategic Placement:** Each piece of user input should be optimally placed into the appropriate DSL section, evaluating the pros and cons of different placements to determine the best DSL section for it.
4. **Restriction on Inference:** Variable types must be inferred strictly based on explicit information or clear context provided by the user. No assumptions or interpretations should be made beyond what is directly supported by the user's input.

### 4. Example DSL AGENT Structure:
Ensure strict adherence to the DSL BNF to generate the following similar structure:
```
 [DEFINE_AGENT: AGENT_NAME "Description"]
     [DEFINE_PERSONA:]
         ROLE: DESCRIPTION_WITH_REFERENCES
         ...
         OptionalAspectName: DESCRIPTION_WITH_REFERENCES
     [END_PERSONA]

     [DEFINE_CONSTRAINTS:]
         ConstraintName: Limitation details
         ...
         OptionalAspectName: DESCRIPTION_WITH_REFERENCES
     [END_CONSTRAINTS]

     [DEFINE_TYPES:]
         SomeType = {
             _attribute_1: str
             ...
         }
     [END_TYPES]

     [DEFINE_VARIABLES:]
```

```
            _var_1: boolean
            _var_2: SomeType
            ...
        [END_VARIABLES]

        [DEFINE_WORKER: "Worker description" WORKER_NAME]
            [INPUTS]
                <REF> _var_name_1 </REF>
                ... # Additional INPUTS if necessary
            [END_INPUTS]

            [OUTPUTS]
                <REF> _var_name_2 </REF>
                ... # Additional OUTPUTS if necessary
            [END_OUTPUTS]

            [MAIN_FLOW]
                [SEQUENTIAL_BLOCK] # SEQUENTIAL_BLOCK example, it's not mean the first block must be the SEQUENTIAL_BLOCK
                    COMMAND-x [COMMAND xxx]
                    ... # Additional COMMANDs
                [END_SEQUENTIAL_BLOCK]

                [kkk_BLOCK DESCRIPTION_WITH_REFERENCES] # NOT SEQUENTIAL_BLOCK example, kkk_BLOCK may be a IF_BLOCK
                    COMMAND-z [COMMAND zzz]
                [END_kkk_BLOCK]

                ... # Additional BLOCK if necessary, e.g., SEQUENTIAL_BLOCK or IF_BLOCK
            [END_MAIN_FLOW]
        [END_WORKER]
    [END_AGENT]
```

Note that all words that are capitalized or underlined are terms in the DSL in the above directives (e.g. DESCRIPTION_WITH_REFERENCES) and they can be found in the DSL BNF.

Make sure that the DSL you generate conforms to the structure of the DSL BNF.
